# Supplementary material for: Neutral theory of cooperative dynamics
Source: arXiv:2506.09737 source file (2025-12-20)
Supplement: Supplementary file 1 [file sm-contents.tex]

% !TeX root = sm.tex

\makeatletter
\renewcommand\section{\@startsection{section}{1}{\z@}%
                                  {-3.5ex \@plus -1ex \@minus -.2ex}%
                                  {2.3ex \@plus.2ex}%
                                  {\fontsize{12pt}{12bp}\selectfont\bfseries\centering}}
\renewcommand\subsection{\@startsection{subsection}{2}{\z@}%
                                  {-3.5ex \@plus -1ex \@minus -.2ex}%
                                  {2.3ex \@plus.2ex}%
                                  {\fontsize{11.5pt}{12bp}\selectfont\bfseries\centering}}

\renewcommand\subsubsection{\@startsection{subsubsection}{3}{\z@}%
                                  {-3.5ex \@plus -1ex \@minus -.2ex}%
                                  {2.3ex \@plus.2ex}%
                                  {\fontsize{11.5pt}{12bp}\selectfont\em\centering}}
\makeatother

\sloppy
\allowdisplaybreaks
\raggedbottom

\onecolumngrid
\setcounter{equation}{0}

% \renewcommand\thesection{\arabic{section}}
% \renewcommand\thesubsection{\arabic{subsection}}
% \renewcommand\thesubsubsection{\arabic{subsubsection}}
% \renewcommand\theequation{S\arabic{equation}}
% \makeatletter 
% %\renewcommand*{\p@subsection}{\thesection.}
% \def\p@subsection     {\thesection.}
% \def\p@subsubsection  {\thesection.\thesubsection.}
%\makeatother 

%\titleformat*{\section}{\fontsize{16}{20}\selectfont} 
%\titleformat*{\subsection}{\fontsize{13}{17}\selectfont}

% \titleformat*{\section}{\fontsize{14}{20}\sffamily\bfseries\selectfont} 
% \titleformat{\subsection}[hang]{\fontsize{12}{17}\sffamily\bfseries\selectfont}{\thesection.\thesubsection}{10pt}{}{}
% \titleformat{\subsubsection}[hang]{\fontsize{11}{15}\sffamily\itshape\selectfont}{\thesection.\thesubsection.\thesubsubsection}{10pt}{}{}
\setcounter{section}{0}

\begin{center}

{\fontsize{15pt}{22bp}\bfseries Supplemental Material:}

\vspace{5pt}
{\fontsize{15pt}{22bp}\bfseries \papertitle }

\vspace{15pt}

{\fontsize{14pt}{15} Jordi Pi\~nero, Artemy Kolchinsky, Sidney Redner and  Ricard Solé }

% \vspace{20pt}
% {\fontsize{15pt}{22bp}\bfseries Supplementary Material }

\end{center}

\fontsize{11pt}{14.5bp}\selectfont
\tableofcontents{}

\fontsize{11pt}{22bp}\selectfont 

\clearpage

% !TeX root = sm.tex

\section{Neutral model of cooperators}
\label{app:set-up}

\subsection{Setup and notation}
\label{subsec:notation}

Our system consists of a well-mixed population of $N$ individuals, 
each belonging to a certain species. Throughout, we use $i,j,\ldots$ as species indices and use $n_i\in\{0,1\ldots,N\}$ to denote the number of individuals belonging to species $i$. 
We use bold symbols to denote population vectors, such as ${\n}=(n_1,n_2,\ldots)$  
for the total number of individuals for each species. Recalling the notation used in the main text, we denote by $R(\n)$ the number of nonzero elements of the vector $\n$, that is, the number of species present in the system. Moreover, if any species becomes extinct
($n_i\to 0$), the species are re-indexed so that the first $R(\n)$ entries of $\n$ are always the strictly positive ones.

Due to our hypothesis of neutrality, all species evolve according to the same rules. 
Without loss of generality, we take $i=1$ to be the {\em representative species}, which, by neutrality, has the same statistical properties as any other species.  In order to alleviate notation, we interchangeably use $n_1\leftrightarrow n$  whenever appropriate.

A central quantity in our analysis is the Simpson index, defined as
\begin{align}
\simp(\n)=\frac{\sum_i n_i^2}{\left(\sum_i n_i\right)^2}=\sum_i\left(\frac{n_i}{N}\right)^2 \,,\label{eq:corrected_Simpson}
\end{align}
where we used $\sum_i n_i = N$. Below, we also refer to the Simpson index of the non-representative species, 
\begin{align}
    \simpnot(\n)=\frac{\sum_{i> 1} n_i^2}{\left(\sum_{i>1}n_i\right)^2}=\sum_{i>1}\left(\frac{n_i}{N-n_1}\right)^2\,.
    \label{eq:lambda-def}
\end{align}
Finally, we denote the steady-state expectation of the Simpson index of all species as $\simpss$, and of the non-representative species as $\simpssnot$.

\subsection{Birth-death process describing the representative species}
\label{subsec:for-back-rates}

In this subsection, we derive a birth-death process (one-dimensional random walk) that describes the stochastic dynamics of $n$, the abundance of the representative species.

\begin{mybox}[label={box:derivationF}]A
{\bf Box I.1: Birth probability}.
In a single timestep, the probability that the representative species undergoes the birth transition $n \to n+1$ is 
\begin{align}
(1-\mig)\left(\frac{n}{N}\right)\left(\frac{N-n}{N}\right)\left(\frac{N-n}{N}\right).
\end{align}
Here, $1-\mig$ is the probability that the timestep involves a replication (rather than migration), $n/N$ is the probability that an individual from the representative species is chosen to replicate, $(N-n)/N$ is the probability that this individual is paired with an individual from a different species, and the final $(N-n)/N$ is the probability that the offspring replaces an individual of a different species.
Since every migration event introduces a {new} species into the system, there is no contribution to the birth probability of the representative species due to migration. 
\end{mybox}

Following from rules {1)} and {2)} in the main text, we derive the birth and death probabilities (see Boxes~\ref{box:derivationF} and \ref{box:derivationB} for a full derivation) as 
\begin{align}
\forward{n}&=(1-\mig)\left(\frac{n}{N}\right)\left(1-\frac{n}{N}\right)^2
\label{eq:forward_rate}\\ 
\backward{n}&=(1-\mig)\left(\frac{n}{N}\right)\left(1-\frac{n}{N}\right)\left[1-\left(1-\frac{n}{N}\right)\simpnot({\n})\right]+\mig
\left(\frac{n}{N}\right) \,.\label{eq:backward_rate}
\end{align}
The birth-death process described by~\eqref{eq:forward_rate}-\eqref{eq:backward_rate}
is not closed. In particular, the death probability $\backward{n}$ depends on all the non-representative species abundances via their respective Simpson index, $\simpnot(\n)$. 
Assuming this Simpson index is tightly concentrated on its steady-state expectation value,  $\simpnot(\n)\approx \simpssnot:=\langle \simpnot(\n)\rangle$, we may approximate steady-state fluctuations by a closed birth-death process:
\begin{align}
\forward{n}&=(1-\mig)\left(\frac{n}{N}\right)\left(1-\frac{n}{N}\right)^2
\label{eq:forward_rate_1d},\\ 
d_{n}&\approx(1-\mig)\left(\frac{n}{N}\right)\left(1-\frac{n}{N}\right)\left[1-\left(1-\frac{n}{N}\right)\simpssnot\right]+\mig
\left(\frac{n}{N}\right), \label{eq:backward_rate_1d}
\end{align}
where we note that $d_n$ now depends only on the abundance of the representative species $n$ and the expected $\simpssnot$.

\begin{mybox}[label={box:derivationB}]A
{\bf Box I.2: Death probability}.
We first consider the probability that, in a given timestep, the representative species undergoes the death transition $n\to n-1$ due to a cooperative interaction. 
Let $B$ and $C$ denote two species different from each other and from $A$ (the representative species). Then, we may have 
$$(B+C)+A \rightarrow
(B+C)+B\quad \text{or} \quad 
(B+A)+ A\rightarrow 
(B+A)+ B,$$  where parentheses denote cooperative interaction. 
Adding up all possible contributions gives
\begin{align}
    &\sum_{i\neq 1}\left(\frac{n_i}{N}\right)\left(\frac{N-n-n_i}{N}\right)\left(\frac{n}{N}\right) + \left(\frac{N-n}{N}\right)\left(\frac{n}{N}\right)\left(\frac{n}{N}\right)\nonumber\\
    &=\left(\frac{N-n}{N}\right)\left(\frac{n}{N}\right)\sum_{i\neq 1}\left(\frac{n_i}{N}\right)
    -\left(\frac{n}{N}\right)\sum_{i\neq 1}\left(\frac{n_i}{N}\right)\left(\frac{n_i}{N}\right)+  \left(\frac{n}{N}\right)\left(\frac{N-n}{N}\right)\left(\frac{n}{N}\right)\nonumber\\
    &=\left(\frac{n}{N}\right)\left[\left(\frac{N-n}{N}\right)\left(\frac{N-n}{N}\right)
    -\sum_{i\neq 1}\left(\frac{n_i}{N}\right)\left(\frac{n_i}{N}\right)+ \left(\frac{N-n}{N}\right)\left(\frac{n}{N}\right)\right]\nonumber\\
    &=\left(\frac{n}{N}\right)\left(\frac{N-n}{N}\right)\left[1-\sum_{i\neq 1}\left(\frac{n_i}{N-n}\right)\left(\frac{n_i}{N}\right)\right]\nonumber \\  
    &=\left(\frac{n}{N}\right)\left(\frac{N-n}{N}\right)\left[1-\left(\frac{N-n}{N}\right)\simpnot(\n)\right],
\end{align}
where in the last line we used definition~\eqref{eq:lambda-def}. In the death  probability~\eqref{eq:backward_rate}, this sum is weighted by $1-\mig$, the probability that a replication event happens in a given timestep. In addition, the death probability includes the term $\mig (n/N)$, representing the probability $\mig$ that an individual of a new species enters the system times the probability $n/N$ that this new migrant replaces 
an individual of the representative species. 
\end{mybox}

\vspace{10pt}

\section{Steady-state species abundance distribution}
\label{app:ss}

In the steady state of a one-dimensional random walk, the detailed balance condition must hold, meaning that birth and death fluxes are balanced:
\begin{align}
    P_nb_n=P_{n+1}d_{n+1},\quad \text{for} \,\,n\in\{1,\ldots,N-1\}\,.
\end{align}
Rearranging, we have that
\begin{align}
    P_n=\frac{b_{n-1}}{d_n}P_{n-1}=\cdots=P_1\prod_{k=1}^{n-1}\frac{b_k}{d_{k+1}}=P_1\frac{\prod_{k=1}^{n-1}b_k}{\prod_{k=2}^nd_k}\,.\label{eq:Pn_expansion}
\end{align}
Using the birth probabilities, Eq.~\eqref{eq:forward_rate_1d}, we may write the numerator on the right-hand side in~\eqref{eq:Pn_expansion} as
\begin{align}
\prod_{k=1}^{n-1}\forward{k} &=\prod_{k=1}^{n-1}(1-\mig)\frac{k}{N}\frac{N-k}{N}\frac{N-k}{N}\nonumber\\
& =\left(\frac{1-\mig}{N^{3}}\right)^{n-1}(n-1)!\frac{\left(N-1\right)!}{\left(N-n\right)!}\frac{\left(N-1\right)!}{\left(N-n\right)!}\,.\label{eq:product-births}
\end{align}
For the death probabilities derived in~\eqref{eq:backward_rate_1d}, it is useful to approximate
\begin{align}
\backward{k} 
& \approx\frac{k}{N}\left[\frac{N-k}{N}\left(1-\frac{N-k}{N}\simpssnot\right)-\mig\frac{N-k}{N}+\mig\right]\nonumber\\
&=\frac{k}{N}\left[\frac{N-k}{N}\left(1-\frac{N-k}{N}\simpssnot\right)+\mig\frac{k}{N}\right]\nonumber\\
 & \approx\frac{k}{N}\frac{N-k}{N}\left(1-\frac{N-k}{N}\simpssnot\right)\nonumber \\
 &=\frac{\simpssnot}{N^{3}}k(N-k)\left(N/\simpssnot-N+k\right).\label{eq:death-prob-approx}
\end{align}
In the first line of~\eqref{eq:death-prob-approx}, we assumed that $\mig\simpssnot\ll1$, which means that at large migration, the system becomes very diverse, and, at small migration, the system retains sufficient diversity. In the second line of~\eqref{eq:death-prob-approx}, we assumed that the system is concentrated on small relative abundances
when $\mig$ is large, thus $\mig (k/N)^2\ll1$.  
Then, the product in the denominator of the right-hand side in~\eqref{eq:Pn_expansion} is approximated as
\begin{align}
\prod_{k=2}^{n}\backward{k} & \approx \left(\frac{\simpssnot}{N^{3}}\right)^{n-1}n!\frac{\left(N-2\right)!}{\left(N-n-1\right)!}\frac{\Gamma\left(N/\simpssnot-N+n+1\right)}{\Gamma\left(N/\simpssnot-N+2\right)}, \label{eq:product-deaths}
\end{align}
where $\Gamma$ indicates Euler's gamma function.

Combining results, and ignoring the factors independent of $n$ (which contribute only to the overall normalization constant), we now compute the ratio in~\eqref{eq:Pn_expansion} as
\begin{align}
P_{n}&\propto \frac{\left(1-\mig\right)^{n}}{n(N-n)}\frac{{\simpssnot}^{-n}}{\left(N-n\right)!\,\Gamma\left(N/\simpssnot-N+n+1\right)}\nonumber
\\
&=\frac{\big(\frac{1-\mig}{1-\simpssnot}\big)^{n}}{n(N-n)}\frac{(1-\simpssnot)^{n}{\simpssnot}^{-n}}{\left(N-n\right)!\,\Gamma\left(N/\simpssnot-N+n+1\right)}\,.
\end{align}
To relate our results to a known probability distribution, we multiply the previous expression by $(1-\simpssnot)^{N/\simpssnot-N}$ and $\Gamma(N/\simpssnot+1)$, which are both independent of $n$, such that
\begin{align}
P_n\propto\frac{\big(\frac{1-\mig}{1-{\simpssnot}}\big)^{n}}{n(N-n)}\frac{\Gamma(N/\simpssnot+1)}{\left(N-n\right)!\,\Gamma\left(N/\simpssnot-N+n+1\right)}(1-\simpssnot)^{N/\simpssnot-N+n}{\simpssnot}^{N-n}.\label{eq:Pn_to_binom}
\end{align}
This way, expression~\eqref{eq:Pn_to_binom} consists of a combination of distributions involving the well-known binomial distribution, though defined using Euler$-\Gamma$ functions instead of factorials:
\begin{align}
    P_n\propto \frac{(1-\mig)^n}{n(N-n)}\frac{\text{Bin}(N-n;N/\simpssnot,\simpssnot)}{(1-\simpssnot)^n},\label{eq:Pn-binom}
\end{align}
where we use notation:
\begin{align}
    \text{Bin}(m;M,p):=\binom{M}{m}p^m(1-p)^{M-m}\equiv\frac{\Gamma(M+1)}{\Gamma(m+1)\Gamma(M-m+1)}p^m(1-p)^{M-m}.
\end{align}
In general, $\text{Bin}(m;M,p)$ refers to binomial distribution over $m\in\{0,\ldots,M\}$ successes, given $M$ total trials and probability of success $p$.

In most cases, we are interested in systems with non-vanishing migration and non-negligible diversity ($\mig>0$ and $1/\simpssnot\gg 1$). In such cases, the steady-state distribution is concentrated on small relative abundances and we may rewrite~\eqref{eq:Pn-binom} by introducing four approximations. First, we estimate the binomial distribution as a discretized Gaussian (ignoring overall constants):
\begin{align}
    \text{Bin}(N-n;N/\simpssnot,\simpssnot)\overset{\sim}{\propto}e^{-n^2/2N}.
\end{align}
Second, when $\simpssnot\ll 1$, we approximate the exponential term $(1-\simpssnot)^{-n}\approx e^{n\simpssnot}$. Third, we take $1/(N-n)\approx 1/N$, which is accurate for $n\ll N$. Finally, we simplify by replacing $\simpssnot$ (the Simpson index of non-representative species) by the expected Simpson index of the entire population:
\begin{align}
    \simpssnot\approx \simpss:=
    \langle \simp(\n)\rangle\,.
\label{eq:simpssnot-eq-simpss}
\end{align}
where $\langle \cdot \rangle$ indicates expectations under the steady-state distribution of abundances $\n$.
Combining the above approximations, we are left with the probability distribution 
reported in Eq.~\eqref{eq:Pn1} in the main text.

\subsection{Quality of the approximation~\eqref{eq:simpssnot-eq-simpss}}

Eq.~\eqref{eq:simpssnot-eq-simpss}, a key step in the  derivation above,  involves two approximations. First, we  approximate the Simpson index of the non-representative species $\simpnot(\mathbf n)$ with the  Simpson index of all species $\simp(\mathbf n)$. Second, we ignore steady-state fluctuations of the Simpson index, approximating $\simp(\mathbf n) \approx \simpss :=\langle \simp \rangle$. In this section, we study the error involved in both approximations.

To consider the approximation $\simpnot(\mathbf n)\approx \simp(\mathbf n)$, we  use the identity
\begin{align}
    N^2\simp = {(N-n)^2 \simpnot + n^2}\,,
\end{align}
where we drop the arguments in $\simp(\mathbf{n})$ and $\simpnot(\mathbf{n})$
for simplicity of notation. It can be rearranged as 
\begin{align*}
N^{2}(\simpnot-\simp) & =2Nn\simpnot-n^{2}(\simpnot+1)\\
(N^{2}-2Nn)(\simpnot-\simp) & =2Nn\simp-n^{2}(\simpnot+1)\,.
\end{align*}
Dividing both sides by $N^{2}\simp$ gives
\[
\left(1-\frac{2n}{N}\right)\frac{\simpnot-\simp}{\simp}=\frac{2n}{N}-\frac{n^{2}}{N^{2}}\frac{\simpnot+1}{\simp}\,.
\]
Next, we drop small terms $2n/N\ll1$ and $\simpnot\ll1$ to give
\[
\frac{\simpnot-\simp}{\simp}\approx\frac{2n}{N}-\frac{n^{2}}{N^{2}}\frac{1}{\simp}\,.
\]
The results described in the main text (and rest of this SI Appendix) imply that  steady-state abundances are concentrated
around $n\approx N\lambda^{*}$. Plugging this in and simplifying
gives
\begin{align}
\frac{\simpnot-\simp}{\simp}\approx\simpss\approx \sqrt{\frac{-\ln (2\pi N \mig^2)}{N}}\,,
\label{eq:appssss}
\end{align}
where we used Eq.~\eqref{eq:ss-div}. For instance, for the system  in Figure~\ref{fig:speciesabundance}(b) ($N=10^5,\mig=10^{-5}$), the relative error is $\approx 0.01$.

Next, we consider the approximation $\simp(\mathbf n) \approx \simpss :=\langle \simp \rangle$ that ignores fluctuations.  
To estimate the scale of the fluctuations of the Simpson index, we use the definition 
\begin{align}
    \simp (\mathbf n) := \sum_{i=1}^R ({n_i}/{N})^2 \,,
\end{align}
where $R$ is the number of species and $n_i$ is abundance of species $i$. 
In the steady state of the low-migration regime, each $n_i$ may be approximated by a Gaussian with mean $N\simpss$ and variance $N$.
Hence $n_{i}/N$ may be approximated as a Gaussian with mean $\simpss$ and variance $1/N$, while  $(n_{i}/N)^{2}$ may be approximated as the square of this Gaussian, which has variance $4\simpss^{2}/N+2/N^2\approx 4\simpss^{2}/N$.
Assuming  that steady-state abundance fluctuations are approximately independent across species,  the fluctuations of $\simp(\mathbf n)$ will have variance 
$ 4 R^*\simpss^{2}/N$.  

The scale of relative fluctuations of $\lambda (\mathbf n)$ are given by the ratio of the standard deviation and the mean, 
${\textrm{Std}(\simp)}/{\simpss}\approx \sqrt{4R^*/N}$. But recall from Eq.~\eqref{eq:Rss} that $R^*=N/\langle n \rangle \approx 1/\simpss$. Combining and using Eq.~\eqref{eq:appssss} gives a simple  estimate of the relative fluctuations:
\begin{align}
   \frac{\textrm{Std}(\lambda)}{\simpss}\approx 
 \frac{2}{\sqrt{\simpss N}}  
 \approx 2^{3/4} (-\ln \mig)^{-1/4} N^{-1/4}  \,.
   \end{align}
For instance, for the system  shown in Figure~\ref{fig:speciesabundance}(b),  $N=10^5$ and $\mig=10^{-5}$ and the size of relative fluctuations  is  $\approx 0.05$.

\vspace{10pt}
\section{Steady-state Simpson index}
\label{app:ss-diversity}

Here we show that the steady-state Simpson index of the system obeys Eq.~\eqref{eq:simpPn} and can be approximated by the expression~\eqref{eq:solA0} given in the main text. 
To begin, we rewrite Eq.~\eqref{eq:corrected_Simpson} as 
\begin{align}
    \simp(\n) =  \sum_{n=1}^N r_n \left(\frac{n}{N}\right)^2 \,
    \label{eq:simp3}
\end{align}
where $r_n$ indicates the number of species with abundance $n$. 
Observe that $\sum_n r_n n=N$, thus $r_n n/N$ is the {fraction} of individuals that belong to the set of species with abundance $n$. The steady-state expectation of $r_n$ is proportional to the probability that the representative species has abundance $n$, that is, $\langle r_n \rangle \propto P_n$. The expected fraction of individuals that belong to the set of species with abundance $n$ is obtained by normalizing as
\begin{align}
\frac{\langle r_n\rangle n}{N}= \frac{P_n n}{\sum_{n} P_{n} n}.
\end{align}
As a sanity check, note that $\sum_n \langle r_n\rangle  n / N =\left\langle\sum_n r_n n\right\rangle /N=1$. Finally, let us take expectation on both sides of~\eqref{eq:simp3} and substitute to give
\begin{align}
\simpss=\langle \simp(\n)\rangle\approx \sum_{n=1}^N\left(\frac{\langle r_n\rangle n}{N}\right)\left(\frac{n}{N}\right)=\frac{1}{N}\frac{\sum_{n=1}^NP_n n^2}{\sum_{n=1}^NP_{n}n},
\label{eq:simpPn-app}
\end{align}
which corresponds to Eq.~\eqref{eq:simpPn} in the main text.
Usefully, the right side is independent of the normalization constant of $P_n$, which is not always easy to compute in practice.

\subsection{Low migration Simpson index}
\label{app:low-migration-simpss}

In the low-migration regime, we can approximate \eqref{eq:simpPn-app} via the Euler-Maclaurin integrals. First, we rewrite our expression for $P_n$, Eq.~\eqref{eq:Pn1}, as
\begin{align}
    P_n\propto \frac{1}{n}e^{-(n-N\simpss)^2/2N+n\ln(1-\mig)}\overset{\sim}{\propto} \frac{1}{n}e^{-\left[n-N(\simpss-\mig)\right]^2/2N},
\end{align}
where we used that, for small migration values, $\ln(1-\mig)\approx -\mig$ and ignored overall constant factors. Then, combining with~\eqref{eq:simpPn-app}, we obtain
\begin{align}
\simpss\approx \frac{1}{N}\frac{\int_1^{N}  e^{-\left[n-N({\simpss}-\mig)\right]^2/2N} n \,dn}{\int_1^{N} e^{-\left[n-N({\simpss}-\mig)\right]^2/2N}dn}\,.\label{eq:simpss-integrals-approximation}
\end{align}
The two integrals can be solved separately. Assuming $N\gg1$,
\begin{align}
    \frac{1}{N}\int_1^{N}  e^{-\left[n-N({\simpss}-\mig)\right]^2/2N} n \,dn&\approx e^{-N(\simpss-\mig)^2/2}+\sqrt{\frac{\pi N}{2}}(\simpss-\mig)\ \erfc\left(\sqrt{\frac{N}{2}}(\mig-\simpss)\right)\nonumber\\
    \int_1^{N} e^{-\left[n-N({\simpss}-\mig)\right]^2/2N}dn&\approx \sqrt{\frac{\pi N}{2}} \erfc\left(\sqrt{\frac{N}{2}}(\mig-\simpss)\right),
\end{align}
where we used the complementary error function, $\erfc(z):=2/\sqrt{\pi}\int_z^{\infty}e^{-t^2}dt$. Combining with~\eqref{eq:simpss-integrals-approximation} yields
\begin{align}
    \simpss \approx \left[\sqrt{\frac{\pi N}{2}}\erfcx\left(\sqrt{\frac{N}{2}}(\mig-\simpss)\right)\right]^{-1}+(\simpss-\mig)\,,\label{eq:simpss-after-integrals-intermediate-step}
\end{align}
where we used the definition of the scaled complementary error function, $\erfcx(z):=e^{z^2}\erfc(z)$. Rearranging~\eqref{eq:simpss-after-integrals-intermediate-step}, we arrive at the result reported in Eq.~\eqref{eq:solA0} from the main text.

\subsection{High migration Simpson index derived from~\eqref{eq:solA0}}
\label{app:high-migration-simpss-from-erfcx}

In the main text, the scaling $\simpss \approx 1/N\mig$ in the high-migration regime ($\mig\gg\simp$) is obtained by re-evaluating~\eqref{eq:simpPn} using the Fisher Logseries distribution. In contrast, here we show that the same result can also be derived from \eqref{eq:solA0}.  
To do so, we may approximate 
\begin{align}
   \erfcx(z)\approx z/[\sqrt{\pi}(z^{2}+1/2)]\quad\text{for} \quad z\to\infty, 
\end{align}
as follows by considering the first two terms of the continued fraction
derived by Laplace~\cite[Livre X, p.~255]{laplace1805traite}. Plugging into \eqref{eq:solA0} and solving gives 
\begin{equation}
\simpss\approx \frac{\mig-\sqrt{\mig^{2}-4/N}}{2}\approx\frac{1}{N \mig}\,,
\end{equation}
where we used our usual assumption that
$N$ is large. 

\vspace{10pt}
\section{Steady-state number of species}
\label{app:num_species}
Here, we derive the expected number of species in steady state, distinguishing between those in the cooperator core, $\Rcore$, and those outside of it, $\Rout$. Our derivation is only valid in the low-migration regime introduced and discussed in Sections~\ref{sec:ss-dist}-\ref{sec:ss-simps} in the main text. The results derived here appear as Eqs.~\eqref{eq:Rcore_estimate} and~\eqref{eq:Rout_estimate} in the main text.

As stated in the main text,  the expected number of species in the core obeys $\Rcore=\Ncore/\expncore$.  
We may use $\Ncore+\Nout=N$ to write
\begin{align}
    \Ncore=N\left(1-\frac{\Nout}{N}\right).
\end{align}
We estimate the fraction of individuals outside the core by
\begin{align}
  \frac{\Nout}{N}=\frac{\sum_{n=1}^{\hat{n}_{\mathsf{min}}}P_n n}{\sum_{n=1}^N P_n n} \approx\frac{\sum_{n=1}^{1/\simpss}e^{-(n-N\simpss)^2/2N}}{\sum_{n=1}^{N}e^{-(n-N\simpss)^2/2N}}\approx \frac{\int_1^{1/\simpss}e^{-(n-N\simpss)^2/2N}}{\int_1^{N}e^{-(n-N\simpss)^2/2N}},
\end{align}
where we used that $\Nout=\sum_{n=1}^{\hat{n}_{\mathsf{min}}}R^*P_n n$ and $N=\sum_{n=1}^N R^* P_n n$, where $R^*$ is the total number of species. We also use that $\hat{n}_{\mathsf{min}}\approx 1/\simpss$, see Eq.~\eqref{eq:nminmax} in the main text. 
We note that the denominator on the right side acts as the normalization constant of the Gaussian probability density function (PDF), which now together with the numerator gives the Gaussian cumulative density function (CDF), often indicated as $\Phi(z)$. Thus, in the large $N$ limit, we write:
\begin{align}
    \frac{\Nout}{N}\approx \Phi\left(\frac{1/\simpss-N\simpss}{\sqrt{N}}\right)\,.
\end{align}
As shown in Eq.~\eqref{eq:ss-div}, for very small migration, $\simpss\gg N^{-1/2}$, which allows us to approximate
\begin{align*}
    \Phi\left(\frac{1/\simpss-N\simpss}{\sqrt{N}}\right)\approx\Phi\left(-N\simpss\right)\approx \Phi(-\infty)=0\,.
\end{align*}
Therefore, to a first approximation, we have that
\begin{align}
    \Ncore=N\left(1-\frac{\Nout}{N}\right)\approx N \,.
\end{align}
Finally, we derive Eq.~\eqref{eq:Rcore_estimate} by combining with 
$\Rcore=\Ncore/\expncore$  and using the approximation $\expncore\approx \hat{n}_{\mathsf{max}}$, with the last term specified in 
Eq.~\eqref{eq:nminmax}.

Regarding the expected number of species 
outside the core, we similarly use $\Rout=\Nout/\expnout$. To proceed, we start by estimating the expected abundance of species outside the core,
\begin{align}
    \expnout &=\frac{\sum_{n=1}^{\hat{n}_{\mathsf{min}}}P_n n}{\sum_{n=1}^{\hat{n}_{\mathsf{min}}}P_n}\approx \frac{\Nout}{N}\frac{\sum_{n=1}^{N}P_n n}{\sum_{n=1}^{1/\simpss}P_n}\,.
    \label{eq:expnout_estimation0}
\end{align}
where, again, we used that $\Nout=\sum_{n=1}^{\hat{n}_{\mathsf{min}}}R^*P_n n$ and $N=\sum_{n=1}^N R^* P_n n$, where $R^*$ is the total number of species. We also use that $\hat{n}_{\mathsf{min}}\approx 1/\simpss$, see Eq.~\eqref{eq:nminmax} in the main text. Rearranging, and substituting $P_n$ by using our main result Eq.~\eqref{eq:Pn1} from the main text, gives

\begin{align}
    \Rout=\frac{\Nout}{\expnout} &\approx \frac{N\sum_{n=1}^{1/\simpss}e^{-(n-N\simpss)^2/2N}/n}{\sum_{n=1}^{N}e^{-(n-N\simpss)^2/2N}}
    ,\label{eq:expnout_estimation}
\end{align} 
We estimate the sum of the denominator in the right-hand side of~\eqref{eq:expnout_estimation} by the Gaussian normalization factor, $\sqrt{2\pi N}$. For the numerator, we approximate
\begin{align}
    \sum_{n=1}^{1/\simpss}\frac{1}{n}e^{-(n-N\simpss)^2/2N}\approx e^{-(1-N\simpss)^2/2N}\sum_{n=1}^{1/\simpss}\frac{1}{n}\approx \sqrt{2\pi N}\mig (-\ln \simpss)\,,
\end{align}
where in the last approximation we evaluated the (slow-changing) exponential term in the range $1\leq n\leq 1/\simpss$ as $e^{-(1-N\simpss)^2/2N}\approx e^{-N\simpss^2/2}\approx \sqrt{2\pi N}\mig$, and then plugged in our estimation of $\simpss$ in the low-migration regime (Eq.~\eqref{eq:solA0} in the main text). Combining the above gives~\eqref{eq:Rout_estimate} as reported in the main text.

\vspace{10pt}
\section{Maximum abundances and the infiltration probability}
\label{app:infiltration-prob}
\subsection{Maximum abundances distribution}
We begin by deriving the probability that a species trajectory (sampled at stationarity) has maximum abundance $m$, which we term $Q_m$. First, we consider the probability that an abundance trajectory with initial value $n$ reaches (or exceeds) abundance $\ell \geq n$ ($\ell\neq 0$). We term this probability $u_n(\ell)$. Second, we derive an analytic expression for $u_1(\ell)$, the probability of reaching (or exceeding) $\ell$ when the trajectory starts at abundance one. Third, we connect results for $u_1$ to $Q_m$ and study the shape of $Q_m$ in the low-migration regime. And fourth, we estimate the \textit{infiltration probability}, i.e., the probability that a trajectory reaches maximum abundance $m\geq N\simpss$.

Consider the probability that a trajectory with initial abundance $n$ reaches (or exceeds) some target abundance $\ell\geq n$ ($\ell\neq 0$) before going extinct. We denote this probability as 
$u_n(\ell)$. We focus in particular on $u_1(\ell)$, which captures the probability that a species that has just migrated into the system reaches (or exceeds) abundance value $\ell>1$. We will focus our analysis on the regime of low migration.  

As described above, our model can be reduced to a birth-death process with transition probabilities $b_n$ and $d_n$, Eqs.~\eqref{eq:forward_rate_1d}-\eqref{eq:backward_rate_1d}. We are also using the approximation $\simp(\n)\approx\simpss$. Then, the probability $u_n(\ell)$ must obey two boundary conditions:
\begin{align}
    u_0(\ell>0)=0\quad \text{and}\quad u_{\ell}(\ell)=1.
\end{align}
The first condition states that the probability of hitting a target once the species has gone extinct ($n\to 0$) is null, while the second condition states that the probability of hitting the target while on target is one. For the values of $n\in\{1,\ldots,\ell-1\}$, the probability $u_n(\ell)$ obeys a recurrence:
\begin{align}
    u_n(\ell)=b_nu_{n+1}(\ell)+d_n u_{n-1}(\ell)+(1-b_n-d_n)u_n(\ell) \,.\label{eq:recurrence-prob-un}
\end{align}
We rearrange~\eqref{eq:recurrence-prob-un} to give:
\begin{align}
    b_n[u_{n+1}(\ell)-u_n(\ell)]=d_n[u_n(\ell)-u_{n-1}(\ell)].\label{eq:recurrence-prob-un1}
\end{align}
We then define the difference $w_n(\ell)=u_n(\ell)-u_{n-1}(\ell)$, which obeys $w_1(\ell)=u_1(\ell)$ since $u_0(\ell)=0$. Then, from~\eqref{eq:recurrence-prob-un1}, we write
\begin{align}
    w_n(\ell)=\frac{d_{n-1}}{b_{n-1}}w_{n-1}(\ell)=\prod_{k=1}^{n-1}\frac{d_k}{b_k}w_1(\ell).
\end{align}
We note that this product is similar to the inverse product obtained in~\eqref{eq:Pn_expansion}, but differs by one in the indexing of the death probability factors. Moreover, since $u_n(\ell)=\sum_{m=1}^n w_m(\ell)$, the recurrence~\eqref{eq:recurrence-prob-un} is solved by
\begin{align}
    u_n(\ell)=\sum_{m=1}^n\prod_{k=1}^{m-1}\frac{d_k}{b_k}u_1(\ell).
\end{align}
We use the condition $u_{\ell}(\ell)=1$ 
to write
\begin{align}
    u_1(\ell)=\left[\sum_{m=1}^{\ell}\prod_{k=1}^{m-1}\frac{d_k}{b_k}\right]^{-1},\label{eq:infiltraiton-prob-exact-enumeration}
\end{align}
which is an exact enumeration for $u_1(\ell)$.

To find a closed-form approximation of Eq.~\eqref{eq:infiltraiton-prob-exact-enumeration} for our model, we recall results~\eqref{eq:product-births},~\eqref{eq:death-prob-approx} and~\eqref{eq:product-deaths}, and carefully rearrange the indices where needed. After some algebra, this results in
\begin{align}
    \prod_{k=1}^{m-1}\frac{d_k}{b_k}\approx \left(\frac{\simpss}{1-\mig}\right)^{m-1}\frac{(N-m)!}{(N-1)!}\frac{\Gamma(N/\simpss - N +m)}{\Gamma(N/\simpss-N+1)}.\label{eq:infiltration-prob-prod-intermediate}
\end{align}
Next, we use the Stirling approximation $\Gamma(z+1)
\approx\sqrt{2\pi } z^{z+1/2} e^{-z}$ (valid for $z\gg 1$), and apply it to each of the terms in~\eqref{eq:infiltration-prob-prod-intermediate}. Expanding terms up to second order in $m/N$, assuming $N\gg 1$ and $\simpss\ll 1$, we reach
\begin{align}
    \prod_{k=1}^{m-1}\frac{d_k}{b_k}\approx \exp\left\{ \frac{m^{2}}{2N}-\left(\simpss+\ln(1-\mig)+\frac{1}{2N}\right)m+\simpss+\ln(1-\mig)\right\}.\label{eq:infiltration-prob-prod-intermediate2}
\end{align}
We now ignore the term $1/2N$ and use the fact that, in the low-migration regime, $\simpss \gg \mig$. This allows us to approximate~\eqref{eq:infiltration-prob-prod-intermediate2} as
\begin{align}
    \prod_{k=1}^{m-1}\left(\frac{d_{k}}{b_{k}}\right)\approx e^{ m^{2}/2N-\simpss (m-1)}
    \,.\label{eq:infiltration-prob-prod-final}
\end{align}
We now plug~\eqref{eq:infiltration-prob-prod-final} back into~\eqref{eq:infiltraiton-prob-exact-enumeration} and for convenience introduce the notation $x_{\ell}:=(\ell-N\simpss)/\sqrt{2N}$. This gives
\begin{align}
    \frac{1}{u_{1}(\ell)}&\approx\intop_1^\ell     \prod_{k=1}^{m-1}\left(\frac{d_{k}}{b_{k}}\right)dm \approx    e^{\ell^2/2N-(\ell-1)\simpss}\left[\sqrt{2N}\DawsonOrig(x_\ell)+\frac{1}{2}\right]-\left[\sqrt{2N}\DawsonOrig(x_1)-\frac{1}{2}\right]
   ,\label{eq:inverse-infiltration-prob}
\end{align}
where we used the Euler-Maclaurin approximation of the sum as an integral plus boundary terms, and ignored terms of order $O(1/N)$ in the exponents. We also  introduced the Dawson function:
\begin{align}
\DawsonOrig(z) := e^{-z^2}\intop_0^z e^{t^2}dt\,.
\end{align}
After a bit of rearranging, we arrive at Eq.~\eqref{eq:u1_inv_n0}, the expression in $u_1(\ell)$ presented in the main text.

\subsection{Bimodality of $Q_m$}

It can be seen from Fig.~\ref{fig:scatter}~(inset) in the main text that the distribution $Q_m$ has a bimodal shape, with a local minimum that separates two modes. 
This allows us to assign species trajectories into two classes: those whose maximum abundance value crosses over the threshold located at the local minimum of $Q_m$ and those that do not. We denote the first set as the \emph{dynamical core}. 

To identify the location of the local minimum of $Q_m$, recall from the main text that $Q_m=u_1(m)-u_1(m+1)$, thus we can approximate $Q_m \approx -{du_1}/{dm}$. Then, the local minimum is given by the condition 
\begin{align}
    0=\frac{d}{dm}Q_m  \approx -\frac{d^2}{dm^2} u_1(m) \propto -2 \left(\frac{d}
{dm}v_m\right)^2+v_m\frac{d^2}{dm^2}v_m \,,
\label{eq:projectbacteriorhodopsin}
\end{align}
where, for notational convenience, we introduced $v_m=1/u_1(m)$ in the right side of Eq.~\eqref{eq:inverse-infiltration-prob}. Considering that equation, it can be shown that the derivatives of $v_m$ become very small at $m=N\simpss$, where the minimum of the exponent's argument is reached. Linearizing the right side of Eq.~\eqref{eq:projectbacteriorhodopsin} around $m\approx N\simpss$ and then solving gives
\begin{align}
    m^*  \approx N\simpss -\frac{1}{2} - \frac{2N-3/4}{ e^{N\simpss^2/2-\simpss} \left( \sqrt{2N} \DawsonOrig(x_1)-1/2\right)+ 1}.    
    \label{eq:jordiishere}
\end{align}
In Eq.~\eqref{eq:x1approx}, we show that $ \sqrt{2N} \DawsonOrig(x_1)\approx -1/\simpss$. Since  $\simpss \gg 1/\sqrt{N}$ in the low-migration regime, the denominator in the last term in Eq.~\eqref{eq:jordiishere} is exponentially large, allowing us to ignore this whole term. We also have $N\simpss \gg 1/2$, thus dropping all sub-dominant terms gives the approximation
\begin{align}
    m^* \approx N\simpss \,.
\label{eq:Qm}
\end{align}

To summarize, we have shown that the maximum abundance distribution $Q_m$  has a local minimum at values of $m \approx N\simpss$.  
Interestingly, the value of this local minimum in $Q_m$ corresponds to the center of the Gaussian contribution to the abundance distribution $P_n$ (Eq.~\eqref{eq:solA0} in the main text) in the low-migration regime. However, this point is not exactly the high-abundance mode of the steady-state distribution, which is located at $\hat{n}_{\mathsf{max}}=N\simpss-1/\simpss$. 

\subsection{Infiltration probability}
Here we derive the infiltration probability to the dynamical core, $\beta$. 
We will use the asymptotic expansion of the Dawson function~\cite[][Eq.~42:6:4]{oldham2009atlas}, 
\begin{align}
    \DawsonOrig(z)=1/(2z) + O(z^{-3}) \qquad \text{for}\qquad \vert z\vert \to \infty \,.
    \label{eq:asymp}
\end{align}

Observe that $\beta$ 
corresponds to the cumulative probability to cross over the local minimum of $Q_m$ located at $N\simpss$:
\begin{align}
    \beta=\sum_{m=N\simpss }^N Q_m=\sum_{m=N\simpss}^N \left[u_1(m)-u_1(m+1)\right]= u_1(N\simpss)-u_1(N)\approx u_1(N\simpss)\,.\label{eq:beta-def-SM}
\end{align}
Here we first used~\eqref{eq:QnUn} from the main text, and then  $u_1(N)\approx 0$. The latter approximation is justified because $u_1(N)\sim e^{-N/2}$ up to polynomial factors, as follows from Eq.~\eqref{eq:inverse-infiltration-prob} and the fact that the Dawson function contributes only polynomial terms, see \eqref{eq:asymp}. To obtain a closed-form expression for $\beta$, we 
substitute back into~\eqref{eq:inverse-infiltration-prob} and keep 
leading-order terms to arrive at
\begin{align}
   \beta \approx \frac{1}{-\sqrt{2N}\DawsonOrig(x_1) }\,.
    \label{eq:beta-full}
\end{align}
Since $x_1 = (1-N\simpss)/\sqrt{2N} \approx -\simpss\sqrt{N/2}\ll -1$ in the low-migration regime, Eq.~\eqref{eq:asymp} implies 
\begin{align}\sqrt{2N}\DawsonOrig(x_1)\approx \sqrt{2N}\DawsonOrig\Big(-\simpss\sqrt{N/2}\Big)\approx -\sqrt{2N}/(\sqrt{2N}\simpss)=-1/\simpss\,,
\label{eq:x1approx}
\end{align}
allowing us to approximate $\beta \approx \simpss$, 
and thus recovering expression~\eqref{eq:beta} from the main text.

\vspace{10pt}
\section{Residence times}
\label{app:mrt}

In this section, we calculate the mean residence time of species whose trajectories reach the dynamical core, as  defined in Section~\ref{app:infiltration-prob} above. 
We also argue that the cooperator core obtained in our study of the steady-state abundance distribution and the dynamical core are effectively equivalent.

At stationarity, let us denote by $T_n$ the mean first passage time (MFPT) from a species with initial abundance $n$ to reach extinction (at abundance $0$). 
We observe that a core species will spend a long time at high abundance values; hence, we assume that the mean residence of a species whose trajectory belongs to the dynamical core can be approximated by the MFPT from $N\simpss$ to extinction,
\begin{align}
   \mrtcore\approx  T_{N\simpss}. \label{eq:mrtcore-to-mfpt}
\end{align}

The MFPT $T_n$ obeys the following recurrence:
\begin{align}
T_{n} = b_{n} T_{n+1} + d_{n} T_{n-1} + (1 - b_{n} - d_{n}) T_{n} + 1.\label{eq:recurrence_Tn}
\end{align}
By defining the differences $V_{n} := T_{n} - T_{n-1}$, this can be rearranged into a first-order recurrence, 
\begin{align}
V_{n} = \frac{d_{n-1}}{b_{n-1}} V_{n-1} - \frac{1}{b_{n-1}}. \label{eq:recurrence_vn}
\end{align}
Recurrence~\eqref{eq:recurrence_vn} is generally solved by
\begin{align}
V_{n} = U_{n-1} V_{1} - W_{n-1}, \quad \text{with} \quad U_{m-1} := \prod_{k=1}^{m-1} \frac{d_{k}}{b_{k}} \quad \text{and} \quad W_{m-1} = \sum_{k=1}^{m-1} \frac{1}{b_{k}} \prod_{j=k+1}^{m-1} \frac{d_{j}}{b_{j}}.\label{eq:vn_solution}
\end{align}

Next, from Eq.~\eqref{eq:infiltration-prob-prod-final} above, 
\begin{align}
U_{m-1} \approx e^{m^{2}/2N - \simpss (m-1)}. \label{eq:U_m-1}
\end{align}
For the other coefficient, we have 
\begin{align}
W_{m-1} = \sum_{k=1}^{m-1} \frac{1}{b_{k}} \prod_{j=k+1}^{m-1} \frac{d_{j}}{b_{j}} = U_{m-1} \sum_{k=1}^{m-1} \frac{1}{b_{k}} \prod_{j=1}^{k} \frac{b_{j}}{d_{j}}.
\end{align}
The expression for $W_{m-1}$ is related to the steady-state distribution $P_{k}$ because 
\begin{align}
P_{k} d_{k} = P_{k-1} b_{k-1} \Rightarrow P_{k} = P_{1} \prod_{j=1}^{k-1} \frac{b_{j}}{d_{j+1}} = d_{1} P_{1} \frac{1}{b_{k}} \prod_{j=1}^{k} \frac{b_{j}}{d_{j}},
\end{align}
therefore we may rewrite $W_{m-1}$ as
\begin{align}
W_{m-1} = \frac{U_{m-1}}{P_{1} d_{1}} \sum_{k=1}^{m-1} P_{k} = \frac{U_{m-1}}{P_{1} d_{1}} C(m-1).
\end{align}
Here, we defined $C(\ell) = \sum_{k=1}^{\ell} P_{k}$, as the cumulative distribution of $P_{k}$ up to $\ell$. Returning now to~\eqref{eq:vn_solution},
\begin{align}
V_{n} = U_{n-1} \left(V_{1} - \frac{1}{P_{1} d_{1}} C(n-1) \right).
\end{align}

At this point, we introduce the boundary conditions of the recurrence~\eqref{eq:recurrence_Tn}. First, we have 
$T_{0} = 0$, which implies $V_{1} = T_{1} - T_{0} = T_{1}$. In addition, we have
\begin{align}
T_{N} = d_{N} T_{N-1} + (1 - d_{N}) T_{N} + 1 \Leftrightarrow d_{N} (T_{N} - T_{N-1}) = 1 \Leftrightarrow V_{N} = \frac{1}{d_{N}}.
\end{align}
The expected number of species in steady state, $R^*$, satisfies the balance equation between 
outflow due to extinction and inflow due to migration:

\begin{align}
\mig = R^{*} P_{1} d_{1},
\end{align}
Recall $d_{N} = \mig$ from Eq.~\eqref{eq:deathprob} in the main text. Put together, these results imply that
\begin{align}
\frac{1}{\mig} = V_{N} = U_{N-1} \left(T_{1} - \frac{R^{*}}{\mig} C(N-1) \right),
\end{align}
which allows us to obtain
\begin{align}
T_{1} = \frac{1}{\mig} \left[ \frac{1}{U_{N-1}} + R^{*} C(N-1) \right] \approx \frac{R^{*}}{\mig}.
\end{align}
Here, we used that, in the low-migration regime, $U_{N-1} \approx e^{N/2 - \simpss N} \gg 1$ in the large $N$ limit, while $C(N-1) \approx 1$ since all the mass is concentrated below $n = N$. Therefore,
\begin{align}
V_{n} \approx \frac{R^{*} U_{n-1}}{\mig} (1 - C(n-1)),
\end{align}
Using the definition of $V_{n}$, the condition $V_1=T_1$, and setting $n=N\simpss$, which is the starting abundance value for our MFPT, then
we have
\begin{align} 
T_{N\simpss} = \sum_{m=1}^{N\simpss} V_{m} \approx \frac{R^{*}}{\mig} \sum_{m=1}^{N\simpss} U_{m-1} \left[1 - C(m-1)\right].\label{eq:Tn_in_terms_of_U_and_C}
\end{align}

Next, we observe that in the low-migration regime, $P_k$ is well-approximated as a Gaussian distribution with mean $N\simpss$ and standard deviation $\sqrt{N}$ (see Eq.~\eqref{eq:Pn1} in the main text). Hence, $C$ is approximated as the cumulative density function of this Gaussian distribution, so $1-C(m-1)\approx 1$ for small $m$ and $1-C(m-1)\approx 1/2$ for $m\approx N\simpss$. On the other hand,  for our range of $m\in[1,N\simpss]\cap\mathbb{N}$, $U_{m-1}$ has a local maximum at $m=1$ and, at small values of $m$,  decays exponentially with rate $1/\simpss$,  
see Eq.~\eqref{eq:U_m-1}. Therefore, in the low-migration regime where $N\simpss^2 \gg 1$, one can verify that as $m$ increases, $U_{m-1}$ decays essentially to 0 while $1-C(m-1)$ remains very close to 1. This allows us to 
approximate:
\begin{align}
    \sum_{m=1}^{N\simpss} U_{m-1} \left[1 - C(m-1)\right]\approx \sum_{m=1}^{N\simpss} U_{m-1}.
\end{align}
The right-hand side corresponds to the expression for $1/u_1(N\simpss)$ that we approximated in~\eqref{eq:inverse-infiltration-prob}. 
Using our approximation of $\beta\approx u_1(N\simpss)$~\eqref{eq:beta-def-SM}, we combine 
with~\eqref{eq:Tn_in_terms_of_U_and_C} to give
\begin{align}
    T_{N\simpss}\approx  
    \frac{R^*}{\mig \beta}.\label{eq:mfpt_dyn-core}
\end{align}
Recall that in the low-migration regime, 
$R^*\approx \Rcore$, which, combined with Eq.~\eqref{eq:Rcore_estimate} in the main text, approximates the MFPT \eqref{eq:mfpt_dyn-core} as
\begin{align}
T_{N \simpss} \approx  \frac{1}{\mig \simpss[1- (N \simpss)^{-1}]}.
\label{eq:mfpt_dyn-core-final}
\end{align}

Result~\eqref{eq:mfpt_dyn-core-final} is equal to our estimate of $\mrtcore$ obtained in Eq.~\eqref{eq:mrtcore} in the main text. This shows that the same  expression for $\mrtcore$ can be derived using two different arguments: a dynamical argument based on the MFPT calculation, and a steady-state argument based on the principle of detailed balance given in Sec.~\ref{sec:dyn} in the main text.
